# Supplementary material for: Does Data-Efficient Generalization Exacerbate Bias in Foundation Models?
Source: arXiv:2408.16154 source file (2024-09-02)
Supplement: Supplementary file 1 [file X_suppl.tex]

\clearpage
\setcounter{page}{1}
\maketitlesupplementary

\section{Rationale}
\label{sec:rationale}

The MEH-MIDAS have images collected from Moorfields Eye Hospital, London, UK between 2000 and 2022, with patients from diverse ethnicities:  British (13.7\%), Indian (14.9\%), Caribbean (5.2\%), African (3.9\%), other ethnicity (37.9\%) and not stated (24.4\%). The Kaggle EyePACS have images from EyePACS in the United States and 3 eye hospitals in India (Aravind Eye Hospital, Sankara Nethralaya, and Narayana Nethralaya) among patients presenting for diabetic retinopathy screening.
